# Supplementary material for: Logic-Q: Improving Deep Reinforcement Learning-based Quantitative Trading via Program Sketch-based Tuning
Source: arXiv:2310.05551 source file (2025-02-06)
Supplement: Supplementary file 1 [file supplementary.tex]

\subsection{Order Execution Setup}
\subsubsection{Datasets \& Training}
We conduct all experiments on the historical transaction data of the stocks of the China A-shares market provided by Fang et al.~\cite{fang2021universal}. The dataset consists of minute-level intraday price-volume market data of CHINA SECURITIES INDEX 800 (CSI 800) constituent stocks and the order amount of each instrument of each trading day. We follow the official implementation~\cite{fang2021universal} and use the data from 2020-09-15 to 2020-11-30 as the training set, 2020-12-01 to 2021-12-31 as the validation set, 2021-01-04 to 2021-01-14 as the test set. For a fair comparison, we use the same training setup as the original implementation~\cite{fang2021universal}. Specifically, the buffer size is set to be 80,000, the training batch size is set to be 1,024, the learning rate is set to be 0.0001 ,and the maximum training epoch is set to be 30. The maximum number of trials of the Bayesian Optimization is set to be 20. The results of the evaluated methods are all averaged over 5 random seeds (same for the stock trading task).
% \lzm{more training hyperparameter settings}
\subsubsection{Compared Methods}
% We conduct all experiments on a server with 48 cores of Intel(R) Xeon(R) Silver 4214 CPU @ 2.20GHz, 4 NVIDIA GeForce RTX 3090 GPUs, and 251G RAM.
We compare our method with two traditional financial
model-based methods and two state-of-the-art DRL methods proposed for order execution.
\begin{itemize}[leftmargin=*]
\item \textbf{Time-Weighted Average Price} (TWAP)~\cite{bertsimas1998optimal}: TWAP is a rule-based method that equally allocates the target order amount into $T$ pieces over the entire trading time horizon.
% and it is the optimal OE strategy under the assumption that market prices adhere to the Brownian motion hypothesis. 
\item \textbf{Volume-Weighted Average Price} (VWAP)~\cite{kakade2004competitive}: VWAP is also a rule-based model that distributes the target order amount to the estimated market transaction volume while monitoring the actual market price. 
\item \textbf{Proximal Policy Optimization} (PPO)~\cite{lin2021end}: PPO is a policy-based DRL strategy based on an agent with a recurrent neural network and is trained with a sparse reward function.
\item \textbf{Oracle Policy Distillation} (OPD)~\cite{fang2021universal}: OPD is a state-of-the-art single-model DRL order execution strategy that utilizes a teacher policy grounded in perfect market information to lead the learning of the target policy.
\item \textbf{Logic-Q}: we implement Logic-Q by using the OPD strategy as the backbone neural policy to demonstrate the effectiveness of Logic-Q for the single-model RL policy.
\end{itemize}
\subsubsection{Evaluation Measurements} 
We evaluate the OE strategies' performance with 4 different measurements:
\begin{itemize}[leftmargin=*]
\item \textbf{Price Advantage} (PA): PA measures the relative gained revenue of a trading strategy compared to a baseline price, formally: $\mathrm{PA}=\frac{10^4}{|\mathbb{D}|} \sum_{k=1}^{|\mathbb{D}|}\left(\frac{p_{s}^k}{p^k}-1\right)$, where $p_{s}^k$ is the average execution price that a strategy achieved on order $k$, $p^k$ is a baseline price (we follow previous work and use the averaged market price of a instrument of a trading day as $p^k$). PA is measured in basis points (BPs), with one basis point equivalent to 0.01\%.

\item \textbf{Additional Annualized Rate of Return} (ARR): ARR measures the additional annualized rate of return brought by an order execution strategy compared to the TWAP strategy.
\item \textbf{Gain-loss Ratio} (GLR): GLR is a metric that compares the average gain from winning trades to the average loss from losing trades over a trading period, formally: $\mathrm{GLR}= \frac{\mathbb{E}[\mathrm{PA} \mid \mathrm{PA}>0]}{\mathbb{E}[\mathrm{PA} \mid \mathrm{PA}<0]}$.
\item \textbf{Positive Rate} (POS): POS measures the positive rate of PA across all orders over a trading period, formally: ${\mathbb{E}[\mathrm{PA}>0]}$. 

\end{itemize}

\subsection{Stock Trading Setup}
\subsubsection{Datasets \& Training} 
For the stock trading task, we conduct experiments on the United States stock market, Hong Kong stock market, and the cryptocurrency market. We use the public dataset collected by Yahoo Finance\footnote{\url{https://github.com/yahoo-finance}}. For the US market, we follow Yang \etal~\cite{yang2020deep} and use the Dow Jones 30 constituent stocks as our trading stock pool, and for the HK market, we use Hang Seng China 50 Index constituent stocks as the trading stock pool.For the cryptocurrency market, we selected cryptocurrencies with significant market volume, including BTC/USD, ADA/USD, FIL/USD, ETH/USD, LTC/USD, BNB/USD, EOS/USD, ETC/USD, LINK/USD, and BCH/USD. We use the public dataset collected by Yahoo Finance\footnote{\url{https://github.com/yahoo-finance}}.
\begin{figure*}[!t] %H为当前位置，!htb为忽略美学标准，htbp为浮动图形
\centering %图片居中
\includegraphics[width=0.85\textwidth]{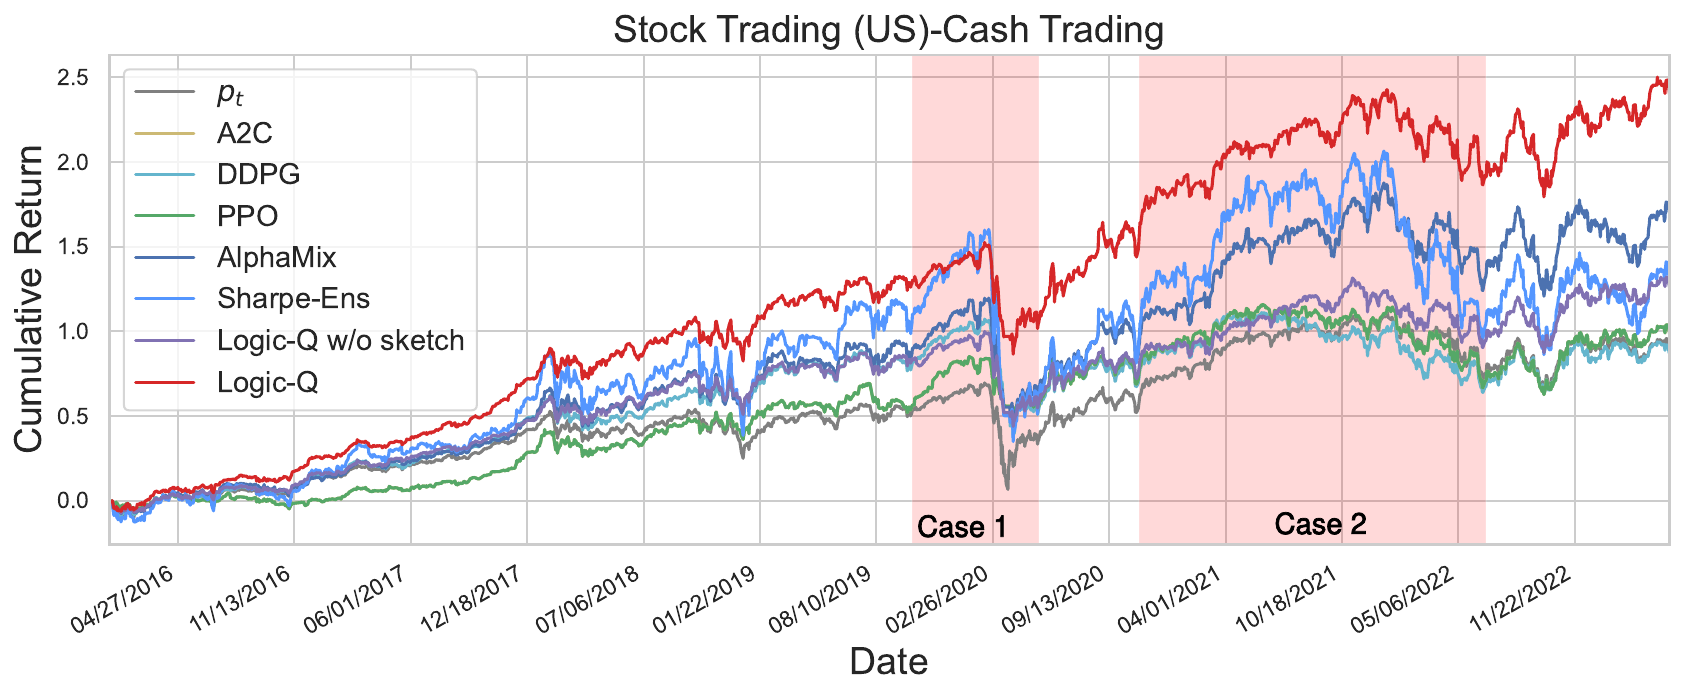} %插入图片，[]中设置图片大小，{}中是图片文件名
% \vspace{-1em}
\caption{Cumulative return curve of different methods for cash trading in the US market} 
% \vspace{-1em}
\label{fig:no_lev} 
\end{figure*}
\begin{figure*}[t] %H为当前位置，!htb为忽略美学标准，htbp为浮动图形
\centering %图片居中
\includegraphics[width=0.85\textwidth]{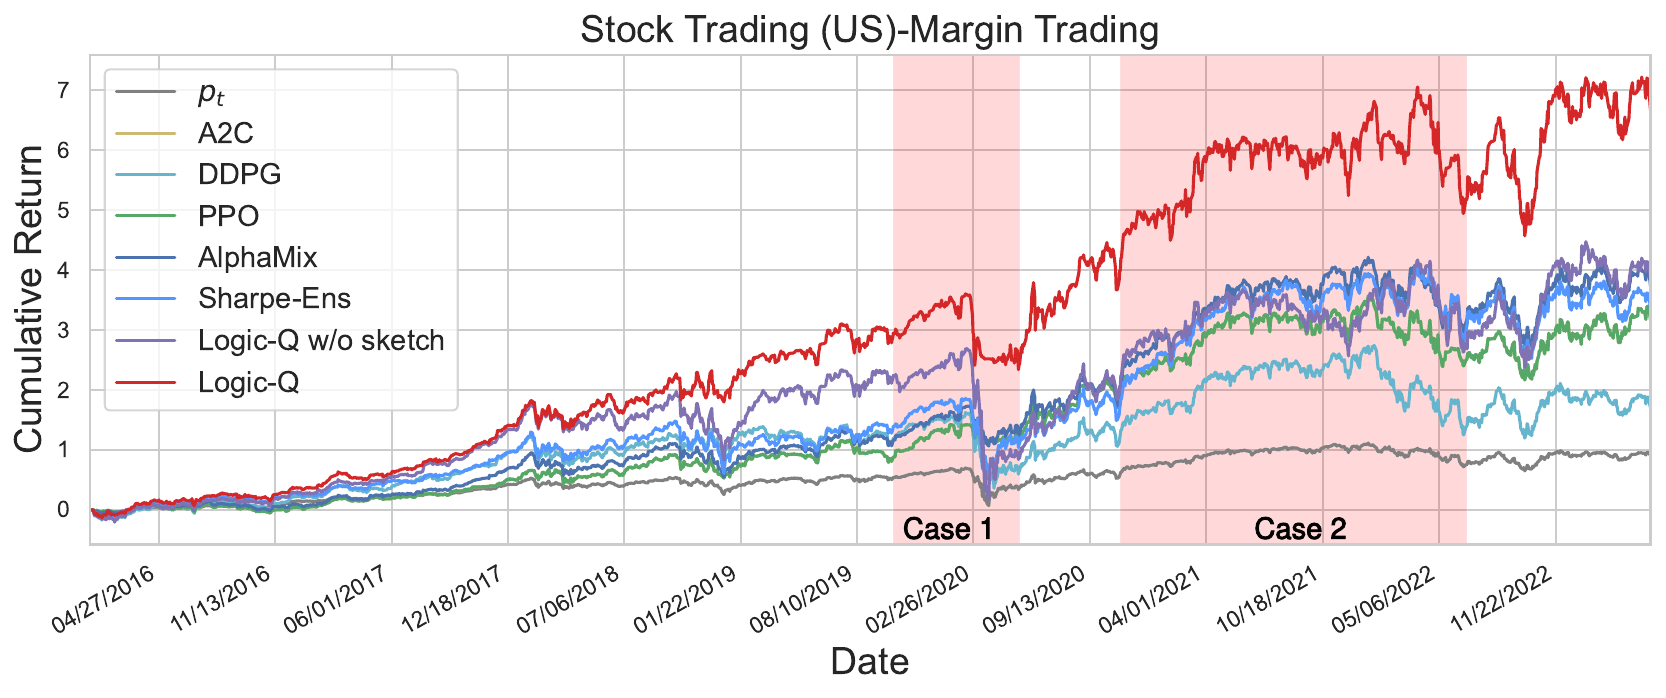} %插入图片，[]中设置图片大小，{}中是图片文件名
% \vspace{-1em}
\caption{Cumulative return curve of different methods for margin trading in the US market} 
% \vspace{-1em}
\label{fig:lev} 
\end{figure*}
Because the cryptocurrency market trades $24$ hours a day, unlike the Hong Kong and U.S. markets, we set an 8-hour trading interval. 
For HK and USA market, We use the daily data from 2009-01-01 to 2015-09-26 as the in-domain training data and the data from 2015-09-26 to 2023-06-01 for validation and testing.
And for cryptocurrency market, We use 8-hours interval data
from 2018-01-01 to 2020-09-25 as the in-domain training data and the data from 2020-09-26 to 2024-05-01 for validation and testing.
Concretely, we follow Yang \etal~\cite{yang2020deep} and use a rolling training-validation-test approach. We recursively update the training-validation-test time step by $3$ months for the US and HK markets, and by $1$ month for the cryptocurrency market, retraining all sub-policies during this period. The initial portfolio value is set at \$1,000,000, with transaction costs at $0.1\%$ of the value of each trade (both buy and sell). The maximum trading volume for a single stock in one day is capped at 100 shares, and for a cryptocurrency within an 8-hour interval, it is limited to \$100,000.

We evaluate Logic-Q and the baselines under both the cash trading and the margin trading scenario. 
For the margin trading setting, we borrow funds equal to the total value of our account, creating a 1:1 loan-to-value ratio. The borrowing amount is adjusted every three months to maintain the same leverage ratio and to repay the interest incurred from borrowing. The interest is calculated based on the borrowed amount and the agreed-upon interest rate with Robinhood\footnote{\url{https://robinhood.com/us/en/support/articles/margin-overview/}} and Binance\footnote{\url{https://www.binance.com/en/fee/marginFee}}. Specifically, for the U.S. and Hong Kong stock markets, we impose an annual margin interest rate of $7.75\%$ for Gold plan subscribers, whereas for the cryptocurrency market, we adopt the Binance VIP3 rate, averaging an annual margin interest of $17.12\%$.
% \lzm{descibe details of leverage, how many times?} 
Our state representation $s\in\mathbb{R}^{331}$ contains 9 major indicators, namely, available balance at the current time step, adjusted close price of each stock, shares owned of each stock, Moving Average Convergence Divergence (\texttt{macd}, \texttt{macds}), Bollinger Bands (\texttt{boll\_ub}, \texttt{boll\_lb}), Relative Strength Index (\texttt{rsi\_30}), Commodity Channel Index (\texttt{cci\_30}), Directional Index(\texttt{dx\_30}), and Simple Moving Average (\texttt{close\_30\_sma}, \texttt{close\_60\_sma}). 

\begin{figure}[!t] %H为当前位置，!htb为忽略美学标准，htbp为浮动图形
\centering %图片居中
\includegraphics[width=0.49\textwidth]{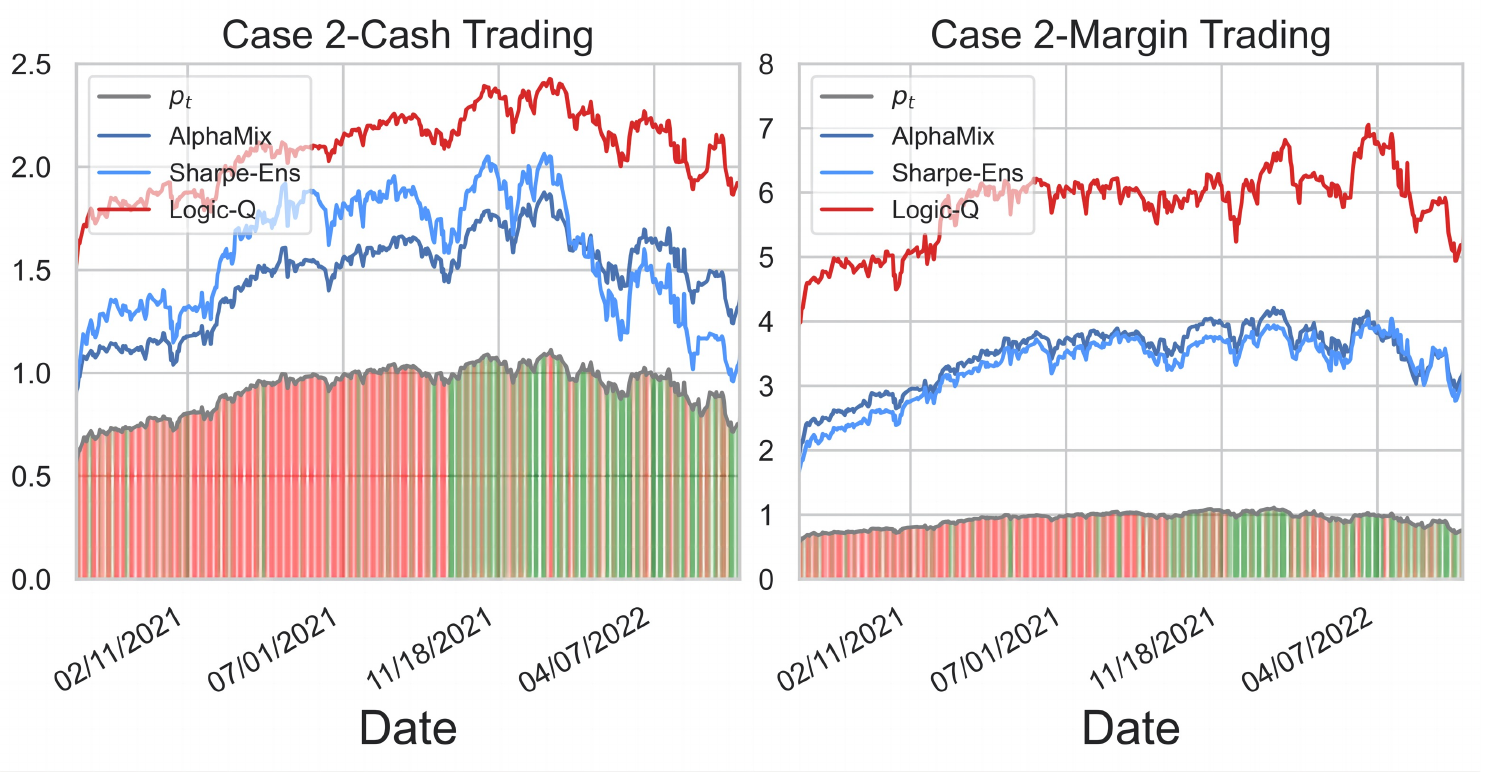} %插入图片，[]中设置图片大小，{}中是图片文件名
% \vspace{-1em}
\caption{Cumulative return curve of different methods in the US market during the Case 2 market crash.} 
% \vspace{-1em}
\label{fig:interpret} 
\end{figure}
\subsubsection{Compared Methods}
\label{sec:st_baselines}
We compare our methods with the following baseline stock trading methods.
\begin{itemize}[leftmargin=*]
\item \textbf{Stock Market Index} ($p_t$): A stock market index is a measure that reflects the performance of the stock market. It is calculated by aggregating the value of a selected group of stocks. We use the Dow Jones Industrial Average (DJIA) for the United States market and we use the Hang Seng China 50 Index (HSI50) for the Hong Kong market~\cite{so2004price}.
\item \textbf{Buy and Hold} (BAH): which is commonly employed to represent the market average and signifies a trading approach where predetermined financial assets are purchased in full at the outset and held until the conclusion of the trading period.

\item \textbf{Deep Deterministic Policy Gradient} (DDPG)~\cite{lillicrap2015continuous}: DDPG is an off-policy DRL algorithm that combines Q-learning~\cite{sutton2018reinforcement} with the policy gradient methods~\cite{sutton1999policy}.
\item \textbf{Advantage Actor Critic} (A2C)~\cite{mnih2016asynchronous}: A2C is an actor-critic-based DRL algorithm that leverages an advantage function to reduce the variance of policy gradient.
\item \textbf{Proximal Policy Optimization} (PPO)~\cite{schulman2017proximal}: PPO is a DRL algorithm that optimizes the policy function using the trust region policy optimization approach. It employs a clipped surrogate objective to prevent large policy updates.
\item \textbf{Sharpe-Ens}~\cite{yang2020deep}: Yang \etal~\cite{yang2020deep} propose this novel ensemble strategy (denoted as Sharpe-ensemble in this paper) which dynamically selects the best-performed DRL agent among a set of candidates according to their Sharpe ratio~\cite{sharpe1994sharpe} on the validation data.
\item \textbf{AlphaMix}~\cite{sun2023mastering}:
Sun \etal~\cite{sun2023mastering} introduce an efficient ensemble learning method to train multiple trading experts with different market trend capabilities, conduct model augmentation from a diversified expert pool, and leverage a three-stage mixture of experts framework to dynamically routing experts from the pool.
\item \textbf{Logic-Q}: we implement Logic-Q by using the Sharpe-Ens strategy as the backbone neural policy to demonstrate the effectiveness of Logic-Q for the ensemble RL policy.
\end{itemize}

\subsubsection{Evaluation Measurements} 
We evaluate the ST strategies' performance with 5 different measurements:
\begin{itemize}[leftmargin=*]
\item \textbf{Annualized return} (AR): Annualized return is a measure of the average annual rate of return on an investment over a specified period. It is calculated by taking the total percentage return of the investment and dividing it by the number of years the investment was held.
\item \textbf{Cumulative return} (CR): Cumulative return is the total amount of return on an investment over a specific period. It is calculated by subtracting the initial investment amount from the final investment value.
\item \textbf{Annualized volatility} (AV): Annualized volatility is a measure of the degree of variation of an investment's returns over a specific period, expressed as an annualized percentage. It is calculated by taking the standard deviation of the investment's returns over the period and multiplying it by the square root of the number of trading days in a year.
\item \textbf{Maximum drawdown} (MD): Maximum drawdown is a measure of the largest percentage decline in the value of an investment from its peak to its trough over a specific period.
\item \textbf{Sharpe ratio} (SR)~\cite{sharpe1994sharpe}: Sharpe ratio is a measure of risk-adjusted return that compares the excess return of an investment over the risk-free rate to its volatility. 
% It is calculated by subtracting the risk-free rate of return from the investment's average annual return, and dividing the result by the investment's standard deviation.
\end{itemize}

\begin{table}[!t]
\centering
\caption{Maximum drawdown of different methods during the Case 2 market crash cases. CT and MT denote cash trading and margin trading respectively.}
\label{tab:md_st}
\begin{tabular}{cc|c|c|c} 
\toprule
Method       & Case 2 CT   & Case 2 MT \\ 
\midrule
$p_t$        & -35.7\%  & -35.7\%  \\
AlphaMix   & -33.8\%  & -30.4\%  \\
Sharpe-Ens  & -53.6\%  & -31.6\%  \\
Logic-Q         & \textcolor{red}{\textbf{-23.1\%}}  & \textcolor{red}{\textbf{-29.9\%}}  \\

\bottomrule
\end{tabular}
% \vspace{-1.5em}
\end{table}
\subsection{Further Investigation}
We further present the cumulative curves of different compared methods under the cash trading and market trading settings in \Cref{fig:no_lev} and \Cref{fig:no_lev}. We can see that Logic-Q can generally outperform the compared methods throughout the period regarding the cumulative return while being resistant to market crashes. Specifically, the two highlighted periods in \Cref{fig:no_lev} and \Cref{fig:lev} denote two market crashes, \Cref{tab:md_st} shows the maximum drawdown of $p_t$, Sharpe-Ens, AlphaMix, and Logic-Q during the two crashes. The results indicate that compared to the previous state-of-the-art methods, Logic-Q presents much lower drawdowns when encountering market crashes. We further present the interpretation analysis of the program sketch for the Case 2 market crash. The results are shown in \Cref{fig:interpret}, and the quantitative results are shown in \Cref{tab:md_st}. Similar to the Case 1 market crash, we can observe that Logic-Q manages to achieve much lower drawdown compared to the state-of-the-art AlphaMix and Sharpe-Ens baselines during the Case 2 market crash. Besides, the market trend identification of the program sketch strongly aligns with human expertise.
